# Supplementary material for: Optimizing for the Shortest Path in Denoising Diffusion Model
Source: arXiv:2503.03265 source file (2025-03-13)
Supplement: Supplementary file 1 [file X_suppl.tex]

% \clearpage
% \setcounter{page}{1}
% \maketitlesupplementary

\label{sec:quali}
\begin{figure}[ht]
\centering
\includegraphics[width=0.9\linewidth]{sd.png}
    \caption{Comparison of our generated panda versus the baseline model’s output. After 3 sampling steps, our model produces a more complete panda with a pinkish hue, closer to the true panda. In contrast, the baseline model generates a sitting panda in 20 steps, while ours follows the prompt to generate a standing panda.}
    \label{figsdlora}
\end{figure}
\section{Additional Results}

In the submitted manuscript, we have thoroughly validated the effectiveness of the proposed method on multiple image denoising benchmarks. To further explore its potential for large models and conduct rapid validation within limited time and computational resources, we carried out a small-scale supportive experiment in the supplementary materials. In this experiment, we selected a small dataset and used a text-to-image generation task for validation.

Specifically, we conducted experiments using Stable Diffusion V1.5 (SDv1.5)\cite{rombach2022high} and LoRA\cite{hu2021lora} as the base models on the Cute Animals\cite{Enflame2024SDTraining} dataset (containing 41 image-text pairs), employing the DDIM\cite{Song2021DDIM} sampler. As shown in Figure \ref{figsdlora}, the panda we generated has colors that are closer to the true panda in the ground truth (GT), with a pinkish hue. After 3 sampling steps, our panda is significantly more complete than the one generated by the original model. In contrast, the original model generated a sitting panda with 20 steps, while ours is standing, which matches the standing prompt. We used Clip Score\cite{hessel2021clipscore} as the evaluation metric and assessed generation quality across different sampling steps, as shown in Table.\ref{tablecs}. From the table, it can be seen that our method shows improvements at all step counts, with more significant improvements for fewer steps (e.g., 2 and 3 steps). This suggests that the proposed method has potential for text-to-image tasks, providing preliminary validation for its application in large models.

\begin{table}[ht] 

\small
\centering
\caption{Clip Score Comparison: A higher Clip Score indicates a better alignment between the generated image and the given text, as it reflects a closer match in the shared semantic space.}
\label{tablecs}
\begin{tabular}{@{}lcccccc@{}}
\toprule
\textbf{Method} & \textbf{2 Steps} & \textbf{3 Steps} & \textbf{5 Steps} & \textbf{20 Steps} \\ \midrule
SDv1.5+LoRA            & 0.588            & 0.749            & 0.843               & 0.855             \\
\hline
\textbf{SDv1.5+LoRA+Ours}     & \textbf{0.610}   & \textbf{0.771}   & \textbf{0.851}             & \textbf{0.856}            \\ \bottomrule
\end{tabular}
\end{table}
